# Supplementary material for: High-fidelity electronic structure and properties of InSb: $G_0W_0$ and Bayesian-optimized hybrid functionals and DFT+$U$ approaches
Source: arXiv:2508.00290 source file (2025-08-01)
Supplement: Supplementary file 1 [file Supplemental_Material.pdf]

# Supplemental information for: "High-fidelity electronic structure and properties of InSb using $G_0W_0$ and Bayesian optimized hybrid and DFT+$U$ methods"

Ritwik Das,[1,2,*] Anne-Sophie Grimault-Jacquin,[1,2] and Frédéric Aniel[1,2]

[1] *Centre for Nanoscience and Nanotechnology (C2N) – French National Centre for Scientific Research (CNRS), Paris, France*

[2] *Université Paris-Saclay, Paris, France*

(Dated: August 1, 2025)

## S1. FORMAL QUASIPARTICLE EXPRESSIONS IN THE $G_0W_0$ APPROXIMATION

In this section, we provide the formal expressions underlying the single-shot quasiparticle ($G_0W_0$) corrections used in the main manuscript.

The self-energy operator in the $GW$ approximation is formally expressed as:

$$\Sigma(\mathbf{r},\mathbf{r}';\omega) = \frac{i}{2\pi}\int d\omega' G_0(\mathbf{r},\mathbf{r}';\omega+\omega')W_0(\mathbf{r},\mathbf{r}';\omega') \tag{S1}$$

where $\Sigma = iGW$ is constructed as the convolution of the noninteracting Green's function $G_0$ and the screened Coulomb interaction $W_0$.

In this framework, the QP energies $\mathcal{E}^{QP}_{n\boldsymbol{k}}$ are obtained by solving the Dyson equation:

$$\left[-\frac{1}{2}\nabla^2 + V_{\text{ion}} + V_H + \Sigma\left(\mathcal{E}^{QP}_{n\boldsymbol{k}}\right)\right]\psi^{QP}_{n\boldsymbol{k}} = \mathcal{E}^{QP}_{n\boldsymbol{k}}\psi^{QP}_{n\boldsymbol{k}} \tag{S2}$$

where $V_{\text{ion}}$ is the ionic potential, $V_H$ is the Hartree potential, and $\Sigma$ replaces the DFT exchange-correlation potential $V_{xc}$. In practice, within the $G_0W_0$ approximation, this equation is solved perturbatively as a first-order correction to the DFT eigenvalues.

The Green's function $G_0$ is given by:

$$G_0(\mathbf{r},\mathbf{r}';\omega) = \sum_{n\boldsymbol{k}} \frac{\psi_{n\boldsymbol{k}}(\mathbf{r})\psi^*_{n\boldsymbol{k}}(\mathbf{r}')}{\omega - \epsilon^{\text{DFT}}_{n\boldsymbol{k}} \pm i\eta} \tag{S3}$$

where $\eta$ is a positive infinitesimal. The screened Coulomb interaction $W_0$ is defined as:

$$W_0(\mathbf{r},\mathbf{r}';\omega) = \int d\mathbf{r}''\, \varepsilon^{-1}(\mathbf{r},\mathbf{r}'';\omega)v(\mathbf{r}'',\mathbf{r}') \tag{S4}$$

* Corresponding author: ritwik.das@universite-paris-saclay.fr; https://ritwikdas.gitlab.io

where $v(\mathbf{r},\mathbf{r}') = 1/|\mathbf{r}-\mathbf{r}'|$ is the bare Coulomb interaction and $\varepsilon^{-1}$ is the inverse dielectric matrix calculated within the random-phase approximation (RPA).

To efficiently capture the frequency dependence of $W_0$, we employ the Godby-Needs plasmon pole model (GPP) [S1], which approximates the full RPA dielectric function with a model featuring a single plasmon pole.

The perturbative correction to the DFT eigenvalues is expressed as:

$$\mathcal{E}^{QP}_{n\boldsymbol{k}} = \epsilon^{\mathrm{DFT}}_{n\boldsymbol{k}} + \langle \psi_{n\boldsymbol{k}} | \Sigma(\epsilon^{\mathrm{DFT}}_{n\boldsymbol{k}}) - V_{xc} | \psi_{n\boldsymbol{k}} \rangle \tag{S5}$$

where $V_{xc}$ is subtracted to avoid double-counting of beyond-Hartree interactions.

## S2. BAYESIAN OPTIMIZATION KERNEL AND MODEL SELECTION

Bayesian optimization (BO) [S2] was employed to optimize the inverse screening length $\mu$ and exchange fraction $\alpha$ in hybrid HSE functionals, and Hubbard $U$ parameter in DFT+U. The optimization was performed using the Gaussian Process Regression (GPR) as a surrogate model from `scikit-optimize` [S3].

A Matern-5/2 kernel was used for the GPR model:

$$K_{\nu=2.5}(x,x') = \sigma^2 \left(1 + \frac{\sqrt{5}d}{l} + \frac{5d^2}{3l^2}\right) e^{-\frac{\sqrt{5}d}{l}}, \tag{S6}$$

where $d = ||x - x'||$ is the Euclidean distance, $l$ is the characteristic length scale, and $\sigma^2$ controls the variance. This kernel balances flexibility and smoothness, making it suitable for computationally expensive functions [S4].

To account for numerical noise in DFT calculations, a WhiteKernel (Eq. (S7)) was included [S4], ensuring robustness against stochastic variations.

$$K_{\mathrm{white}}(x,x') = \sigma_n^2 \delta(x,x'), \tag{S7}$$

where $\sigma_n^2$ represents the noise variance, and $\delta(x,x')$ is the Kronecker delta function.

The optimization framework employed an adaptive acquisition function strategy, dynamically selecting among Expected Improvement (EI), Probability of Improvement (PI), and Lower Confidence Bound (LCB) at each iteration [S5, S6]:

i. **Expected Improvement (EI):** Prioritizes points with high expected reduction in the objective function.
ii. **Probability of Improvement (PI):** Selects points likely to outperform the current best solution.
iii. **Lower Confidence Bound (LCB):** Trades off exploration and exploitation by adjusting a confidence-weighted criterion.

Each function was weighted dynamically based on prior optimization performance to ensure efficient convergence. Hyperparameters, including the kernel length scale $l$, were optimized via Maximum Likelihood Estimation (MLE)

within the `skopt` framework. This approach effectively minimized the number of expensive first-principles evaluations while maintaining high accuracy.

## S3. DETAILED ANALYSIS OF LDA AND GGA BAND STRUCTURES

In this section, we provide a detailed comparison of electronic band structures calculated using the local density approximation (LDA) and generalized gradient approximation (GGA) exchange-correlation (XC) functionals (Fig. S1). Band structures computed without (Figs. S1a, c) and with (Figs. S1b, d) explicitly including the semicore $4d$ electrons in the valence states (for both the In and Sb atoms) demonstrate significant differences, highlighting the limitations inherent in these widely-used XC functionals.

Without inclusion of the semicore $4d$ electrons, both LDA and GGA (PBE) functionals yield qualitatively correct band ordering at the $\Gamma$-point. LDA (Fig. S1a) produces a direct band gap ($E_0 = 0.191$ eV) that underestimates the experimentally measured gap (approximately 0.235 eV at 0 K), reflecting the well-known band-gap underestimation intrinsic to LDA. Similarly, the GGA-PBE functional (Fig. S1c) predicts a slightly larger band gap ($E_0 = 0.388$ eV) than LDA, yet it still deviates notably from the experimental value due to the same fundamental underestimation of quasiparticle energies by semilocal functionals.

The inclusion of highly localized semicore $4d$ states as explicit valence electrons in the pseudopotential dramatically exacerbates these shortcomings. With the semicore $4d$ electrons explicitly considered, both LDA (Fig. S1b) and GGA-PBE (Fig. S1d) functionals fail to accurately reproduce even the qualitative band ordering and character around the valence band maximum (VBM). Specifically, LDA with $4d$ electrons (Fig. S1b) incorrectly predicts a zero band gap at the $\Gamma$-point due to the inversion of the light-hole (LH) band above the heavy-hole (HH) band, eliminating the fundamental gap entirely. This unphysical band inversion is highlighted explicitly in the figure (red annotated area). Similarly, GGA-PBE with semicore states (Fig. S1d) also reduces the band gap to zero and significantly alters the valence-band splitting and curvature, again demonstrating unphysical LH-HH splitting behavior.

The origin of these issues lies in the substantial repulsion between the semicore $4d$ orbitals and valence $5p$ orbitals, notably Sb-$5p$, which shifts valence band states upwards in energy. This shift severely modifies orbital hybridization at the top of the valence band, resulting in incorrect energy ordering, exaggerated spin-orbit splitting, and the artificial band inversion that removes the fundamental band gap entirely. Such incorrect predictions highlight severe limitations of standard LDA and GGA treatments, particularly when semicore electrons with strongly localized orbitals must be explicitly treated as valence electrons. These shortcomings necessitate higher-level corrections, such as hybrid functionals or explicit Hubbard corrections (DFT+$U$), to achieve physically accurate band structures, as demonstrated clearly in the main manuscript through comparison with experiments and more accurate quasiparticle GW results.

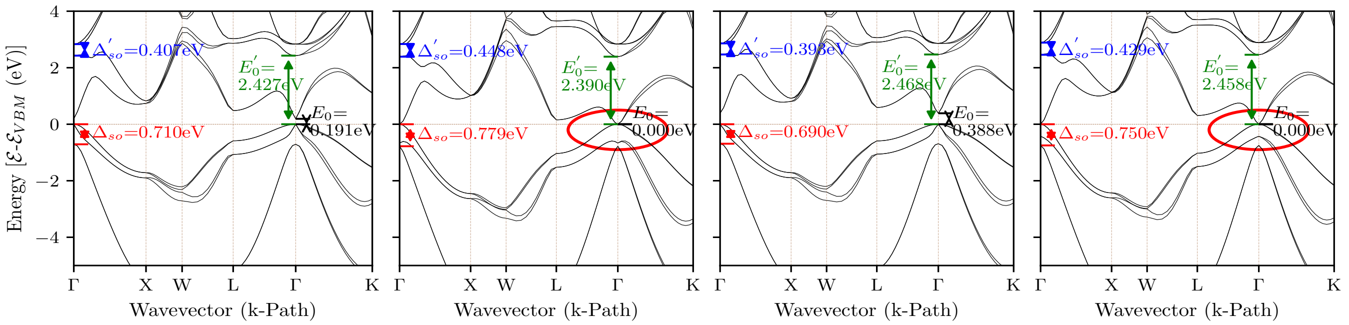


(a) LDA (PAW) without 4*d* (b) LDA (PAW) with 4*d* (c) PBE (PAW) without 4*d* (d) PBE (PAW) with 4*d*

FIG. S1: Electronic band structures of InSb calculated using (a,b) LDA and (c,d) GGA-PBE XC functionals. Results without (a,c) and with (b,d) explicit semicore 4*d* states in the valence configuration are shown. The red highlighted areas emphasize the unphysical heavy-hole and light-hole (HH-LH) splitting (b,d) and the band inversion at the Γ-point (b), causing zero band gaps and incorrect qualitative electronic structures when 4*d* electrons are explicitly treated as valence states for both In and Sb atoms.

## S4. HUBBARD $U$ OPTIMIZATION AND ATOMIC ORBITALS

The DFT+$U$ correction is applied selectively to the 5*p* orbitals of In and Sb, guided by *ab initio* and data-driven reasoning about orbital localization and their contribution to electronic structure. Two Bayesian optimization configurations were used, based on the dimensionality of the optimization space:

i. **1D**: optimizing a single $U$ value for Sb-5*p* states;

ii. **2D**: simultaneously optimizing $U$ values for both In-5*p* and Sb-5*p* orbitals.

The rationale for targeting only the 5*p* states lies in their dominant contribution to the band edges: the valence band maximum (VBM) is primarily composed of Sb-5*p* orbitals, while the conduction band minimum (CBM) has strong In-5*p* character. These orbitals exhibit moderate spatial localization and hybridization in zinc blende (ZB) InSb, making them susceptible to self-interaction errors in semilocal functionals like GGA (PBE, PSEsol). Applying a Hubbard correction to these orbitals improves band edge positioning and dispersion, enhancing agreement with GW and experimental benchmarks.

Although the In-4*d* semicore states lie well below the VBM (approximately 14-17 eV), they are explicitly included as valence in all our PAW and ONCV pseudopotentials. This ensures that *p*-*d* repulsion—especially between In-4*d* and Sb-5*p* states–is properly captured. However, for the final production, we do *not* apply a Hubbard $U$ correction to the In-4*d* states. This choice is based on both physical reasoning and quantitative evidence:

a. **Energy Separation and Localization:** In-4*d* states are deeply bound and well localized, showing negligible hybridization with band-edge states. Their spectral position is already well captured by GGA functionals.

b. **No Need for Correction:** These semicore states do not suffer from delocalization errors. Applying a positive $U_{\text{In-4d}}$ rigidly shifts them downward in energy (and upward with negative $U_{\text{In-4d}}$), with no improvement in band structure accuracy or gap predictions as seen in Fig. S3.

c. **Impact on Spectral Features:** As illustrated in Fig. S3(a-e), sweeping $U_{\text{In-4d}}$ from −5 to +5 eV (with $U_{\text{Sb-5p}}$

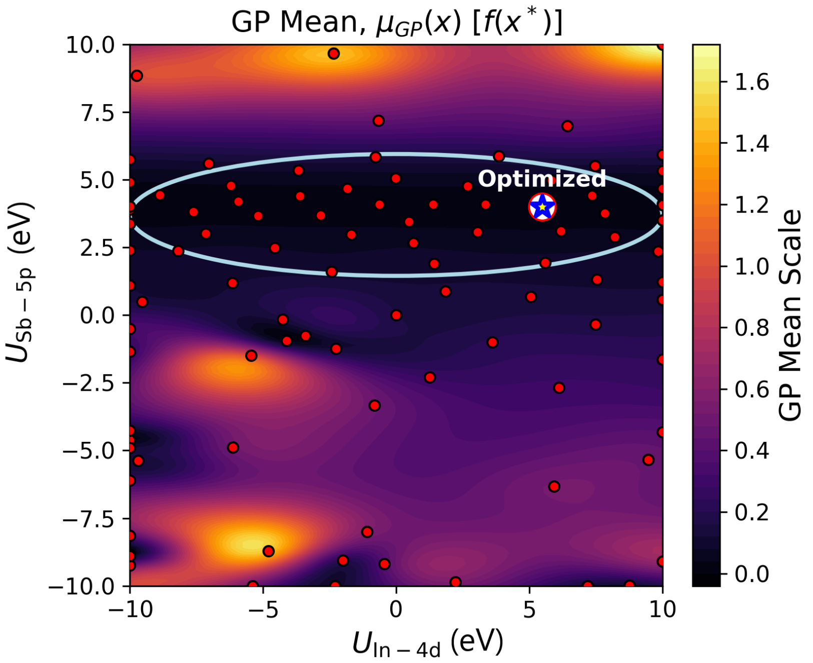


FIG. S2: 2D Gaussian process (GP) posterior mean surface obtained during Bayesian optimization over $U_{\text{In-4d}}$ and $U_{\text{Sb-5p}}$. Red dots indicate evaluated points; the blue star marks the optimal parameters. The elongated, flat dark band running horizontally across the $U_{\text{In-4d}}$ axis (highlighted by the white oval) indicates that the objective function is largely insensitive to $U_{\text{In-4d}}$ in this region. In contrast, sharper variation along $U_{\text{Sb-5p}}$ signifies its much stronger influence on model performance.

fixed at 3.84 eV) pushes the In-4$d$ bands from around $\approx -11$ to $\approx -17$ eV. No significant changes are observed in band gap, $\Delta_{\text{SO}}$, demonstrating that the correction has little relevance to low-energy.

d. **Data-Driven Evidence from BO-GP Mean Surface:** Figure S2 presents the 2D Gaussian process (GP) posterior mean surface from Bayesian optimization over $U_{\text{In-4d}}$ and $U_{\text{Sb-5p}}$. A wide, flat dark region spans horizontally across the $U_{\text{In-4d}}$ axis—highlighted by the white oval—indicating that the objective function value remains nearly unchanged over a broad range of $U_{\text{In-4d}}$ (from $-10$ to $+10$ eV), and between $U_{\text{In-5p}} \in [1.8, 5.8]$ eV. This flatness suggests that the model accuracy is insensitive to the value of $U_{\text{In-4d}}$ within this range, i.e., the BO process is effectively indifferent to corrections on In-4$d$. In contrast, the objective function shows a pronounced minimum along the $U_{\text{Sb-5p}}$ axis, confirming the critical role of Sb-5$p$ correction in determining band gap accuracy and spectral features.

e. **Alignment with Literature:** Prior studies on In-based III-V semiconductors, including those using GW and hybrid-DFT, also omit $U$ corrections on In-4$d$, despite including these states in the valence space [S7, S8].

To summarize, while the inclusion of In-4$d$ in the valence space is essential for physical accuracy, applying an explicit $U$ correction to these states is neither necessary nor helpful. Both physical insight and BO-GP data confirm that $U_{\text{In-4d}}$ is a weakly sensitive parameter, whereas $U_{\text{In-5p}}$ plays a critical role. Our optimized 2D DFT+$U$ model, focusing on relevant 5$p$ orbitals, achieves excellent predictive performance without overfitting or spectral distortion.

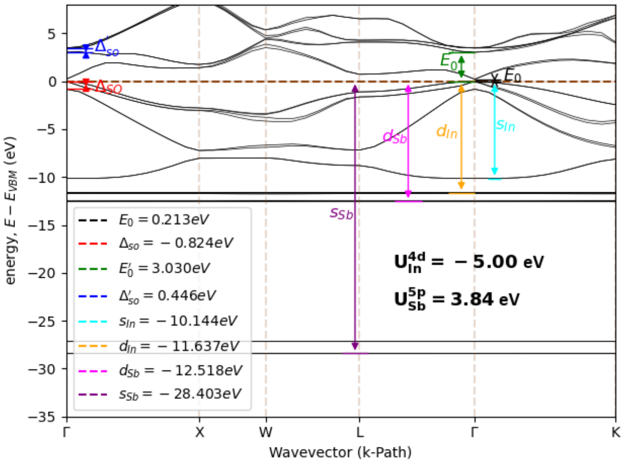


(a) $U^{4d}_{\mathrm{In}} = -5.00$ eV

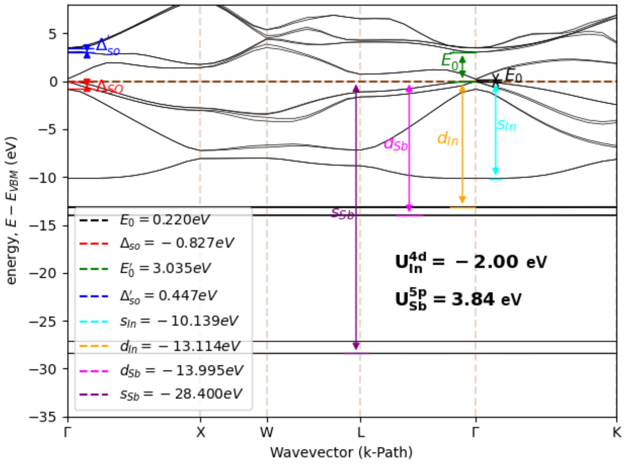


(b) $U^{4d}_{\mathrm{In}} = -2.00$ eV

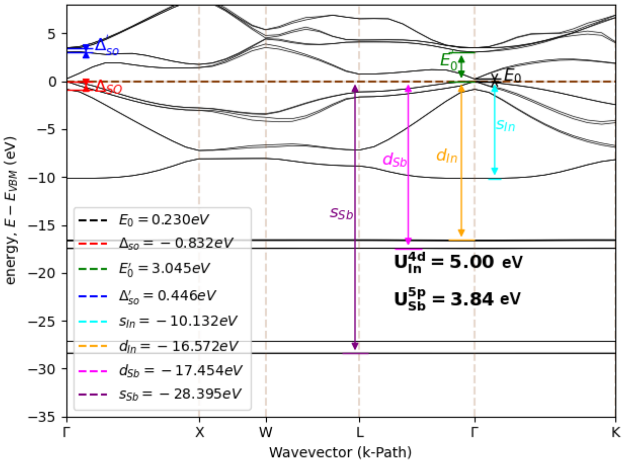


(c) $U^{4d}_{\mathrm{In}} = 5.00$ eV

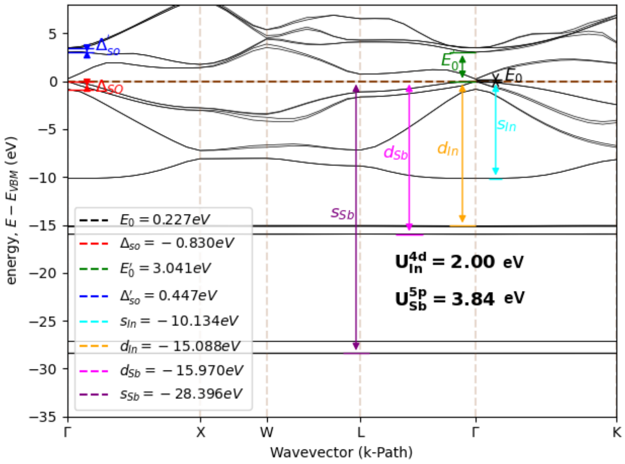


(d) $U^{4d}_{\mathrm{In}} = 2.00$ eV

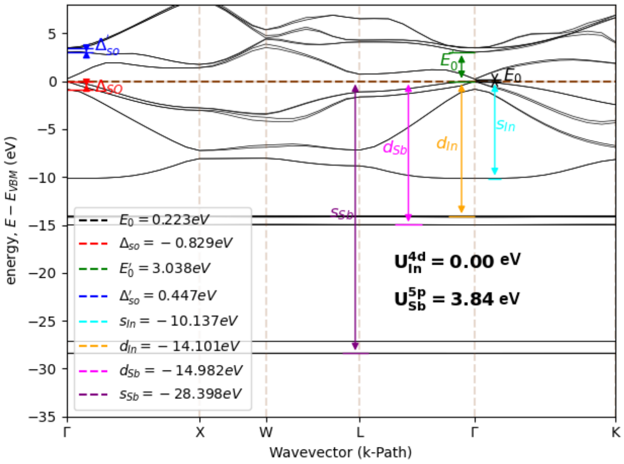


(e) $U^{4d}_{\mathrm{In}} = 0.00$ eV

FIG. S3: Band structures for InSb at fixed $U^{5p}_{\mathrm{Sb}} = 3.84$ eV and varying $U_{\text{In-4d}}$. In-4$d$ levels shift downwards monotonically with increasing $U$, while the low-energy band gap and dispersion remain nearly unchanged.

## S5. DETAILED VALIDATION OF PARAMETER TRANSFERABILITY UNDER HYDROSTATIC STRAIN

To comprehensively validate the transferability of our Bayesian-optimized parameters, specifically the Hubbard parameter ($\boldsymbol{U_{eff}}$) for DFT+$U$ (PBEsol+$U$-$J$) and the hybrid exchange fraction ($\boldsymbol{\alpha}$) for $\mathrm{HSEsol_{HFmix}}$, we systematically analyzed the orbital-projected electronic band structures of InSb under various hydrostatic strain conditions ($\varepsilon_h = -2\%, 0\%, +1\%, +2\%$).

Under hydrostatic compression ($\varepsilon_h = -2\%$), the lattice constant decreases, leading to shorter In-Sb bond lengths and stronger orbital overlap. This enhanced orbital hybridization raises the conduction-band minimum (CBM), which remains dominated by In-5$s$ states, and concurrently lowers the valence-band maximum (VBM), predominantly composed of Sb-5$p$ states. Consequently, the direct band gap at the Γ-point increases significantly, preserving the direct-gap semiconducting character of InSb. This behavior is correctly reproduced by our transferred optimized parameters, indicating their robustness under compressive conditions.

At equilibrium (no strain, $\varepsilon_h = 0\%$), the electronic structure reflects standard InSb characteristics: the CBM predominantly exhibits In-5$s$ orbital character, while the VBM is chiefly derived from Sb-5$p$ states. Here, both methods (DFT+$U$ and $\mathrm{HSEsol_{HFmix}}$) precisely recover experimental and previously established theoretical band gaps and orbital distributions, validating their optimization under equilibrium conditions.

As tensile strain is applied ($\varepsilon_h = +1\%$), lattice expansion reduces the orbital overlap, modifying the effective hybridization between the In-5$s$ and Sb-5$p$ orbitals. Under these conditions, the CBM and VBM energies approach each other, shrinking the fundamental band gap. With further tensile strain ($\varepsilon_h = +2\%$), the orbital mixing between conduction and valence states intensifies, eventually leading to a distinct band inversion at the Γ-point. Specifically, the Sb-5$p$ states shift upwards energetically, surpassing the In-5$s$ conduction states, resulting in an inverted electronic band structure – a hallmark of strain-induced topological transitions. This inversion closely aligns with predictions from advanced theoretical methods reported previously by Feng et al. [S9].

Figure S4 explicitly illustrates these strain-driven transitions using projected band structures obtained from PBEsol+$U$(1D). Panels (a,e) clearly indicate the strong separation of In-5$s$ and Sb-5$p$ orbital contributions at $\varepsilon_h = -2\%$, maintaining the band-gap character. At equilibrium (b,f), this separation remains evident. As tensile strain progresses (c,g), clear orbital mixing emerges, indicating initial stages of hybridization-induced band-gap narrowing. Ultimately, at $\varepsilon_h = +2\%$ (d,h), pronounced orbital intermixing and inversion are observed, directly confirming the robustness and predictive accuracy of our transferred Bayesian-optimized parameters under significantly altered structural conditions.

The robustness of these parameters across a broad range of strain conditions confirms their reliability in predicting the electronic structure of III-V semiconductors under structural perturbations without re-optimization. Additionally, the predictive capability of these parameters has also been successfully demonstrated for alloyed systems ($\mathrm{InAs}_x\mathrm{Sb}_{1-x}$), further establishing their broader applicability, as will be reported in detail in a separate manuscript currently in preparation.

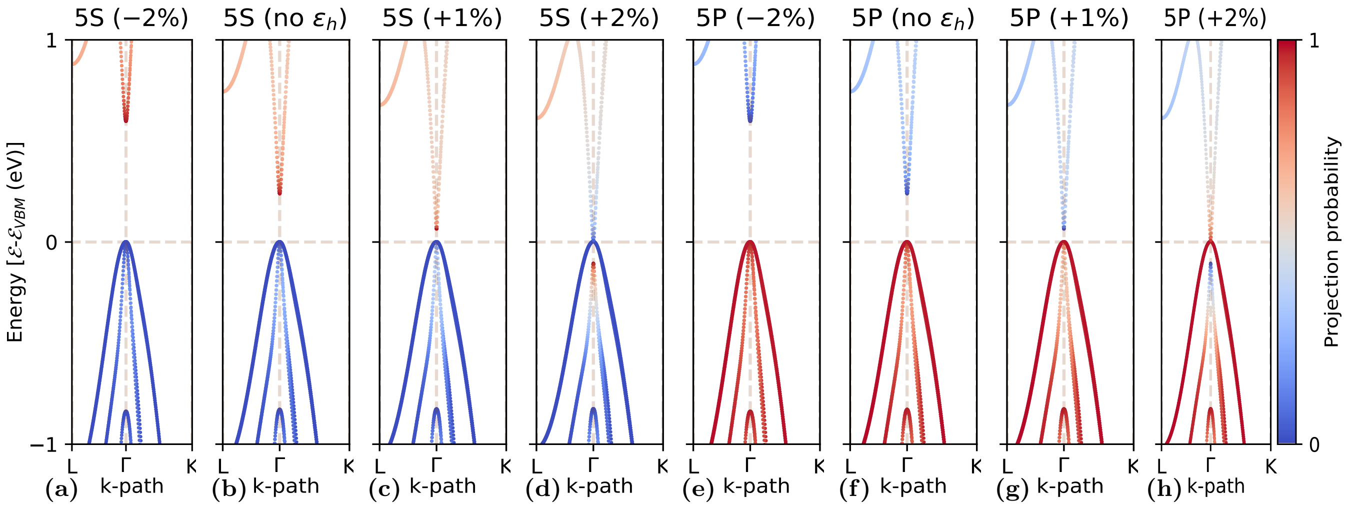


FIG. S4: PBEsol+$U$-$J$(1D) projected electronic band structures of InSb under hydrostatic strain calculated using optimized $\boldsymbol{U_{eff}}$ parameters transferred from bulk calculation. Orbital contributions shown: In-5$s$ (a-d) and Sb-5$p$ (e-h). Strain conditions: (a,e) $\varepsilon_h = -2\%$, (b,f) equilibrium $\varepsilon_h = 0\%$, (c,g) tensile $\varepsilon_h = +1\%$, and (d,h) tensile $\varepsilon_h = +2\%$. The evolution of band gap closure and inversion under tensile strain matches previous theoretical predictions [S9], highlighting the excellent transferability and reliability of the optimized parameters.

## S6. COMPUTATIONAL COST ANALYSIS

The computational cost of electronic structure methods varies significantly with the underlying formalism, implementation, and system size. For hybrid functionals like HSE06 and its screened variants, the inclusion of nonlocal Fock exchange leads to an asymptotic scaling between $O(N^3)$ and $O(N^4)$, depending on the use of fast Fourier transforms (FFT), real-space screening, and parallelization efficiency. For the 2-atom primitive cell of InSb, HSE calculations in this work were observed to be 100–4000× more expensive than GGA or DFT+$U$ calculations, with costs increasing with denser $\boldsymbol{k}$-point meshes and tighter convergence thresholds.

The $G_0W_0$ method introduces even higher computational demands. Beyond the initial HSE06 mean-field calculation, $G_0W_0$ requires construction of the dielectric matrix $\boldsymbol{\varepsilon(\omega)}$ and self-energy $\boldsymbol{\Sigma}$, both of which depend on a large number of unoccupied states and dense $\boldsymbol{k}$- and $\boldsymbol{q}$-grids. The overall scaling ranges from $O(N^4)$ to $O(N^6)$ depending on the approach (e.g., plasmon-pole approximation vs. full-frequency, analytic continuation, and Coulomb truncation). In our InSb calculations, we find $G_0W_0$ to be approximately 10–100× more expensive than HSE and up to $10^4\times$ more expensive than DFT+$U$ for equivalent convergence accuracy. Reducing number of empty bands and using a coarser $\boldsymbol{k}$-point grid significantly reduces the cost of $G_0W_0$, but at the expense of quasiparticle accuracy.

Bayesian optimization of $U_{eff}$ involves 60–100 self-consistent DFT+$U$ calculations for the bulk InSb system. While each DFT+$U$ calculation involves diagonalization and FFT-based steps that scale roughly between $O(N^{2.5})$ and $O(N^3)$ depending on the pseudopotentials and parallelization, the total optimization remains tractable. The combined cost is ∼70–100× that of a single DFT+$U$ run – still orders of magnitude cheaper than a single HSE or $G_0W_0$ calculation.

While $G_0W_0$ delivers benchmark accuracy, its computational overhead limits its applicability mostly to small systems. HSE-based methods offer a compromise between cost and accuracy, especially when parameters like $\boldsymbol{\alpha}$ and

$\boldsymbol{\mu}$ are optimized. In contrast, DFT+$U$—when calibrated via Bayesian optimization—emerges as an efficient and accurate alternative, particularly well-suited for large supercells, disordered alloys, and exploratory high-throughput studies.

---

[S1] R. W. Godby and R. J. Needs, Metal-insulator transition in Kohn-Sham theory and quasiparticle theory, Physical Review Letters **62**, 1169 (1989).

[S2] R. Das, BMach: a Bayesian machine for optimizing Hubbard U parameters in DFT+U with machine learning (2024), arXiv:2407.20848 [cond-mat, physics:physics].

[S3] T. Head, M. Kumar, H. Nahrstaedt, G. Louppe, and I. Shcherbatyi, Scikit-optimize, Zenodo (2024).

[S4] C. E. Rasmussen and C. K. I. Williams, *Gaussian Processes for Machine Learning*, 3rd ed., Adaptive Computation and Machine Learning (MIT Press, Cambridge, Mass., 2008).

[S5] D. R. Jones, M. Schonlau, and W. J. Welch, Efficient Global Optimization of Expensive Black-Box Functions, Journal of Global Optimization **13**, 455 (1998).

[S6] N. Srinivas, A. Krause, S. M. Kakade, and M. Seeger, Gaussian Process Optimization in the Bandit Setting: No Regret and Experimental Design, IEEE Transactions on Information Theory **58**, 3250 (2012), arXiv:0912.3995 [cs].

[S7] L. R. Brennaman and A. J. Samin, Insights into the performance of InAs-based devices in extreme environments from multiscale simulations, Applied Physics A **129**, 1 (2023).

[S8] M. Yu, S. Yang, C. Wu, and N. Marom, Machine learning the Hubbard U parameter in DFT+U using Bayesian optimization, Nature (npj) Computational Materials **6**, 1 (2020).

[S9] W. Feng, W. Zhu, H. H. Weitering, G. M. Stocks, Y. Yao, and D. Xiao, Strain tuning of topological band order in cubic semiconductors, Physical Review B **85**, 195114 (2012).
